# Supplementary material for: Reproduction of the charge density wave phase diagram in $1T$-$\mathrm{TiSe}_2$ exposes its excitonic character
Source: arXiv:1712.04967 source file (2018-11-30)
Supplement: Supplementary file 1 [file TiSe2-excins-si.pdf]

— **Supplementary Information** —

# Reproduction of the charge density wave phase diagram in 1T-$TiSe_2$ exposes its excitonic character

Chuan Chen,[1,2] Bahadur Singh,[1,2] Hsin Lin,[3] and Vitor M. Pereira[1,2,*]

[1] *Centre for Advanced 2D Materials and Graphene Research Centre, National University of Singapore, Singapore 117546*

[2] *Department of Physics, National University of Singapore, Singapore 117542*

[3] *Institute of Physics, Academia Sinica, Taipei 11529, Taiwan*

(Dated: November 30, 2018)

## CONTENTS

S-I. The CDW as an excitonic instability 4
S-I.A. Mean field calculation on the exitonic instability 4
S-I.B. Stability of CDW phase with doping and temperature 5
S-I.C. Bare and exciton-renormalized bandstructure 7
S-I.D. Validity of the single valence band approximation 8
S-I.E. Mapping chemical potential to doping introduced by Cu intercalation 10

S-II. Electron-phonon coupling and electron-electron interaction 12
S-II.A. Mean-field description of the CDW with both excitons and phonons 12
S-II.B. Estimating the lattice distortion in the excitonic-condensed state 14

S-III. The lattice instability *ab-initio* 14
S-III.A. Details of the DFT calculations 14
S-III.B. Renormalized band structure: Mexican hat features 16
S-III.C. GGA and HSE band structure of normal and distorted phase 17
S-III.D. Unfolded bands with and without doping or distortion 18
S-III.E. Effective mass from ARPES and DFT calculations 20
S-III.F. Phonon hardening with Cu doping 20
S-III.G. Robustness of the PLD and CDW transition with smearing function 22

S-IV. Pertinence of studying a monolayer for the bulk system 23

Supplementary References 26

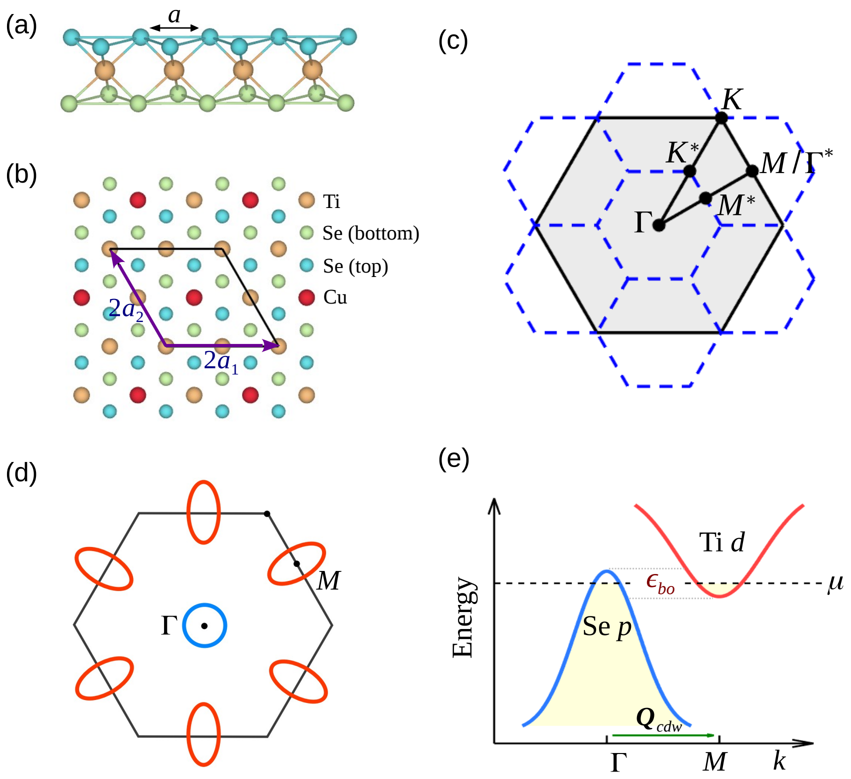


FIG. S1. Crystal structure, Brillouin zone, and bare band topology of the $TiSe_2$ monolayer. (a) 1T phase with octahedral prismatic local structure of Ti and Se atomic layers. (b) Top view of the $TiSe_2$ monolayer with Cu doping. The black rhombus identifies the $2 \times 2$ supercell and red balls show the Cu atoms which lie above the central Ti atoms in the supercell. $\boldsymbol{a_1}$ and $\boldsymbol{a_2}$ are the primitive vectors in the normal phase $(1 \times 1)$. (c) BZ of the normal $(1 \times 1$, solid black) and distorted $(2 \times 2$, dashed blue) phases, where the points marked with $*$ refer to the reduced Brillouin zone. (d) The Fermi contours and (e) schematic band structure near $E_F$ in the normal phase. The Se-derived valence band has its maximum at $\Gamma$ while the Ti-derived electron pockets are centered at the $\boldsymbol{M}$ points. Their overlap is quantified by $\epsilon_{bo}$ and $\Gamma\text{M} = \mathbf{Q}_{\text{cdw}}$.

# S-I. THE CDW AS AN EXCITONIC INSTABILITY

## S-I.A. Mean field calculation on the exitonic instability

We formulate the mean field theory using the equation of motion method. The interaction in the Hamiltonian (1) is decoupled in the particle-hole channel as

$$c^\dagger_{\boldsymbol{k}+\boldsymbol{q},\sigma} d_{i,\boldsymbol{k}',\sigma'} = \delta_{\boldsymbol{k}+\boldsymbol{q},\boldsymbol{k}'}\delta_{\sigma,\sigma'}\langle c^\dagger_{\boldsymbol{k}',\sigma} d_{i,\boldsymbol{k}',\sigma}\rangle + \left[c^\dagger_{\boldsymbol{k}+\boldsymbol{q},\sigma} d_{i,\boldsymbol{k}',\sigma'} - \delta_{\boldsymbol{k}+\boldsymbol{q},\boldsymbol{k}'}\delta_{\sigma,\sigma'}\langle c^\dagger_{\boldsymbol{k}',\sigma} d_{i,\boldsymbol{k}',\sigma}\rangle\right], \tag{S1}$$

$$d^\dagger_{i,\boldsymbol{k}'-\boldsymbol{q},\sigma'} c_{\boldsymbol{k},\sigma} = \delta_{\boldsymbol{k}+\boldsymbol{q},\boldsymbol{k}'}\delta_{\sigma,\sigma'}\langle d^\dagger_{i,\boldsymbol{k},\sigma'} c_{\boldsymbol{k},\sigma}\rangle + \left[d^\dagger_{i,\boldsymbol{k}'-\boldsymbol{q},\sigma'} c_{\boldsymbol{k},\sigma} - \delta_{\boldsymbol{k}+\boldsymbol{q},\boldsymbol{k}'}\delta_{\sigma,\sigma'}\langle d^\dagger_{i,\boldsymbol{k},\sigma} c_{\boldsymbol{k},\sigma}\rangle\right], \tag{S2}$$

so that, by neglecting the product of the fluctuation (bracketed) terms, we achieve the mean-field Hamiltonian

$$H_{\mathrm{MF}} \equiv \sum_{\boldsymbol{k},\sigma,i} \varepsilon_{v\boldsymbol{k}} c^\dagger_{\boldsymbol{k},\sigma} c_{\boldsymbol{k},\sigma} + \varepsilon_{c\boldsymbol{k},i} d^\dagger_{i,\boldsymbol{k},\sigma} d_{i,\boldsymbol{k},\sigma} - \sum_{\boldsymbol{k},\sigma,i} \Delta_{i,\boldsymbol{k},\sigma} c^\dagger_{\boldsymbol{k},\sigma} d_{i,\boldsymbol{k},\sigma} - \Delta^*_{i,\boldsymbol{k},\sigma} d^\dagger_{i,\boldsymbol{k},\sigma} c_{\boldsymbol{k},\sigma} + \frac{1}{\mathcal{N}} \sum_{i,\sigma} \sum_{\boldsymbol{k},\boldsymbol{k}'} V_{i,\boldsymbol{k}-\boldsymbol{k}'} \langle c^\dagger_{\boldsymbol{k},\sigma} d_{i,\boldsymbol{k},\sigma}\rangle \langle d^\dagger_{i,\boldsymbol{k}',\sigma} c_{\boldsymbol{k}',\sigma}\rangle, \tag{S3}$$

where the order parameter

$$\Delta_{i,\boldsymbol{k},\sigma} \equiv \frac{1}{\mathcal{N}} \sum_{\boldsymbol{k}'} V_{i,\boldsymbol{k}-\boldsymbol{k}'} \langle d^\dagger_{i,\boldsymbol{k}',\sigma} c_{\boldsymbol{k}',\sigma}\rangle \tag{S4}$$

gives a measure of the Fourier component at wavevector $\mathbf{Q}_{\mathrm{cdw}}$ of the charge density. In passing, we note the formal analogy between (S3) and (S4), and the equations that describe the SC order parameter in a multi-band $s$-wave semiconductor within a BCS theory. How the magnitude of $V$ is mentioned in the main text. Also, since all terms in (S3) are spin-diagonal, they will be suppressed in the expressions henceforth, but are implicit in all the results.

The theory is developed in terms of Matsubara Green's functions[1] which requires the definition of normal and anomalous propagators as the $\tau$-ordered thermal averages

$$\mathcal{G}_v(\tau,\boldsymbol{k}) = -\langle \mathcal{T}\, c_{\boldsymbol{k}}(\tau) c^\dagger_{\boldsymbol{k}}(0)\rangle, \tag{S5a}$$

$$\mathcal{D}_{j,i}(\tau,\boldsymbol{k}) = -\langle \mathcal{T}\, d_{j,\boldsymbol{k}}(\tau) d^\dagger_{i,\boldsymbol{k}}(0)\rangle, \tag{S5b}$$

$$\mathcal{F}_i(\tau,\boldsymbol{k}) = -\langle \mathcal{T}\, d_{i,\boldsymbol{k}}(\tau) c^\dagger_{\boldsymbol{k}}(0)\rangle, \tag{S5c}$$

which are straightforwardly seen to obey the following coupled equations of motion (in Matsubara frequency space, $i\omega_n$):

$$(i\omega_n - \varepsilon_{v\boldsymbol{k}})\,\mathcal{G}_v(\omega_n, \boldsymbol{k}) + \textstyle\sum_i \Delta_i \mathcal{F}_i(\omega_n, \boldsymbol{k}) = 1, \tag{S6a}$$

$$(i\omega_n - \varepsilon_{c\boldsymbol{k},i})\,\mathcal{F}_i(\omega_n, \boldsymbol{k}) + \Delta_i^* \mathcal{G}_v(\omega_n, \boldsymbol{k}) = 0, \tag{S6b}$$

$$(i\omega_n - \varepsilon_{c\boldsymbol{k},j})\,\mathcal{D}_{j,i}(\omega_n, \boldsymbol{k}) + \Delta_j^* \mathcal{F}_i^\dagger(\omega_n, \boldsymbol{k}) = \delta_{j,i}, \tag{S6c}$$

$$(i\omega_n - \varepsilon_{v\boldsymbol{k}})\,\mathcal{F}_i^\dagger(\omega_n, \boldsymbol{k}) + \textstyle\sum_j \Delta_j \mathcal{D}_{j,i}(\omega_n, \boldsymbol{k}) = 0. \tag{S6d}$$

There are 16 coupled equations in the set (S6) because $i, j \in \{1, 2, 3\}$, which are to be solved to obtain the order parameter

$$\Delta_{i,\boldsymbol{k}} = \frac{k_B T}{\mathcal{N}} \sum_{\boldsymbol{k}',\omega_n} V_{i,\boldsymbol{k}-\boldsymbol{k}'} e^{i\omega_n 0^+} \mathcal{F}_i^\dagger(\omega_n, \boldsymbol{k}'). \tag{S7}$$

The $C_3$ symmetry relating the dispersion of the three conduction bands [Fig. S1(d)] and our approximation of dropping the $\boldsymbol{q}$-dependence in $V_{i,\boldsymbol{q}}$ make the order parameter independent of both $\boldsymbol{k}$ and $i$, allowing one to set $\Delta \equiv \Delta_{i,\boldsymbol{k}}$. From equations (S6) one obtains

$$\Delta + \frac{k_B T}{\mathcal{N}} \sum_{\boldsymbol{k}',\omega_n} \frac{A\,V\Delta}{|\Delta|^2 B - C} = 0, \tag{S8}$$

with

$$\begin{aligned}
A \equiv& (i\omega_n - \varepsilon_{c,2})(i\omega_n - \varepsilon_{c,3}),\\
B \equiv& (i\omega_n - \varepsilon_{c,2})(i\omega_n - \varepsilon_{c,3}) + (i\omega_n - \varepsilon_{c,1})(i\omega_n - \varepsilon_{c,3})\\
&+ (i\omega_n - \varepsilon_{c,1})(i\omega_n - \varepsilon_{c,2}),\\
C \equiv& (i\omega_n - \varepsilon_{c,1})(i\omega_n - \varepsilon_{c,2})(i\omega_n - \varepsilon_{c,3})(i\omega_n - \varepsilon_v),
\end{aligned}$$

and all the $\varepsilon_{c,i}$ and $\varepsilon_v$ are evaluated at $\boldsymbol{k}'$.

It is worth noting that this equation can also be obtained by minimizing the free energy functional $\mathcal{F}[\Delta]$, which is usually formulated within a path-integral formalism. In other words, Eq. (S8) is equivalent to $\partial F[\Delta]/\partial\Delta = 0$, which will be a useful identification below to establish the order of the transition to the excitonic/CDW phase.

### S-I.B. Stability of CDW phase with doping and temperature

The degree of band overlap is seen to be quantitatively important but not qualitatively matter in the sense that a small overlap still stabilizes a broken symmetry phase with a sizeable $T_c$ (e.g., when

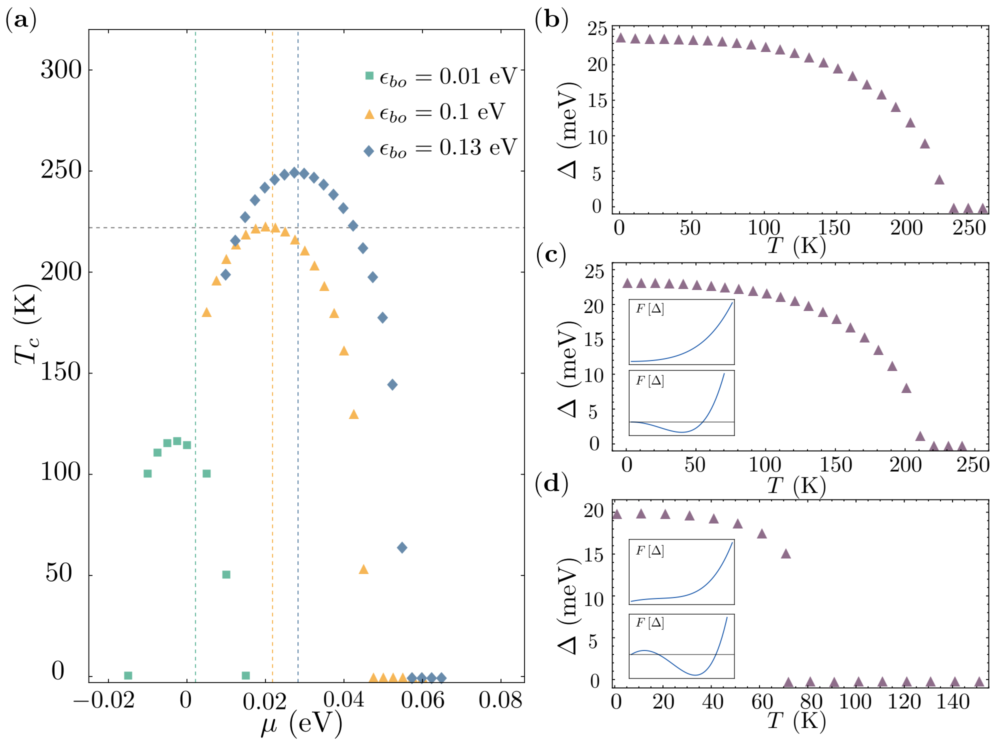


FIG. S2. The CDW phase transition in $TiSe_2$ according to the excitonic instability alone. (a) Critical temperature ($T_c$) as a function of chemical potential ($\mu$) for different levels of overlap between the electron and hole pockets, $\epsilon_{bo}$. Zero in the horizontal scale corresponds to $\mu$ coinciding with the bottom of conduction pockets. The vertical dashed lines indicate the energies where the bare electron and hole pockets intersect for each case. It is clear that, while small variations in $\mu$ tend to quickly reduce $T_{\rm c}$, variations in the band overlap have a less significant effect. (b-d) Temperature dependence of the excitonic order parameter, $\Delta(T)$, at different doping: (b) $x = 0$, (c) $x = 0.003$, and (d) $x = 0.042$. The top (bottom) insets in (c) and (d) show the behavior of the free energy as a function of order parameter for $T > T_c$ ($T < T_c$), and illustrate that the transition becomes of first order in our calculation beyond $x \gtrsim 0.038$.

$\epsilon_{bo}$ is reduced 10-fold, the optimal $T_{\rm c}$ is decreased by only 50 % to 100 K). Physically, this relative robustness is a sensible outcome because the electronic instability is governed here primarily, not by the number of carriers in each pocket, but by the density of states (DOS) at the point of band intersection in the folded zone. Since the CDW gap opens at that intersection (and not at $\mu$ unlike the BCS problem; see supplementary Fig. S3), the CDW phase is most favorable when $\mu$ coincides with the band intersection, and progressively weakens when the system is doped in either direction [the intersection energy is signaled by the vertical dashed lines in Fig. S2(a), which correlates with the optimal $T_{\rm c}$]. In fact, being such a defining characteristic of the excitonic instability, the existence of an optimum $T_{\rm c}$ directly correlated with $\mu$ at the intersection of the conduction and valence

pockets can provide a clear experimental confirmation of a strong excitonic character associated with the CDW instability. Therefore, experimental confirmation of whether this mechanism is critical or not in driving the CDW instability in $TiSe_2$ and closely related TMDs can be obtained by probing $T_c$ as a function of both electron and hole doping, to establish: (i) whether or not an optimal $T_c$ exists and (ii) whether it indeed correlates with the pocket intersection. The latter can be identified either by the doping dependence of ARPES spectra or first-principles bandstructure calculations similar to the ones described below. While different pristine systems might have $\mu$ naturally above or below the pocket crossing point due to natural doping, the optimal situation should be achievable by deliberate substitution in one direction or the other.

To scrutinize the nature of the phase transition in more detail, we show the temperature dependence of the order parameter in panels (b-d) of Fig. S2. Whereas at low doping we have a clear $2^{\mathrm{nd}}$ order transition [Fig. S2(b,c)], above $x \approx 0.038$ it evolves to $1^{\mathrm{st}}$order. The insets illustrate schematically the behavior of the corresponding free energy at $T \gtrsim T_c$ and $T \lesssim T_c$. It is physically very significant that this crossover occurs at the densities where ICDW begin to develop experimentally. The fact that the transition becomes of $1^{\mathrm{st}}$ order can be taken as indication of an underlying tendency for phase segregation at $x \gtrsim 0.038$, or that the commensurate state is not the true ground state, one of whose outcomes can certainly be the experimentally observed discommensurations beyond this level of doping[2]. It is noteworthy that our calculation assumes a commensurate CDW from the outset and cannot describe the incommensurate regime. Yet, it predicts its extinction at the doping level where experiments cease to observe a strictly commensurate phase (in other words, the calculation describes both $T_c(x)$ and $x_c$ for the commensurate phase extremely well).

### S-I.C. Bare and exciton-renormalized bandstructure

Fig. S3 shows two representative cases of the bare and renormalized bandstructures that result from the self-consistent solution of the excitonic order parameter. The two different band overlaps ($\epsilon_{bo} = 0.1$ eV and $\epsilon_{bo} = 0.01$ eV) were chosen to illustrate the cases of large and small overlap. The dispersion curves are plotted in the reduced ($2 \times 2$ folded) Brillouin zone as a function of $k_y$ near the folded $\Gamma$ point. There are always 3 conduction and one valence bands. The chemical potential ($\mu$, dashed gray line at $E = 0$) is set at the value that corresponds to the highest transition temperature for each case (see Fig. S2).

It is worth noting that, whereas at $\epsilon_{bo} = 0.1$ eV the optimal $\mu$ defines both electron and hole pockets in the bare bands, for small band overlap ($\epsilon_{bo} = 0.01$ eV) the optimal $\mu$ lies slightly below

the bottom of the bare conduction bands and in the gap of the interaction-corrected bandstructure. We remark also the resemblance between the shape of the interaction-corrected bands shown here and the bandstructure obtained by DFT in the relaxed $2 \times 2$ distorted phase plotted in Fig. S5.

Perhaps the qualitatively most significant aspect of the CDW transition as seen from the perspective of this excitonic instability is the partial suppression of electronic states below $T_c$. It is evident in the representative case of Fig. S3(b) that one of the electron pockets is removed with the development of a Mexican hat shaped highest conduction band above $\mu$ (inset). This entails a sharp drop in the number of conduction electrons as the temperature decreases through $T_c$ (see also the next section and Fig. S4 below). Simultaneously, the hole pocket disappears as well in the CDW phase, as is clear from the fact that the valence band in Fig. S3(b) (which is shaped like an inverted Mexican hat) is pushed down below the chemical potential. Therefore, according to these results and the physics of the excitonic instability, while in the normal state ($T > T_c$) the transport properties of $TiSe_2$ are determined by both electrons and holes, when the system enters the CDW state electrons become the majority carriers (holes get suppressed), albeit with an overall smaller electron density on account of the partial loss of electronic states. This is consistent with the well known fact that, experimentally, both Hall effect, Seeback coefficient, and magnetic susceptibility[3,4] show a clear transition to electron-like transport as $T$ is lowered below $T_c$. For example, undoped samples ($x = 0$) of $TiSe_2$ have a reproducibly positive Hall constant for $T > T_c$, which drops to zero at $T_c$ and becomes steeply negative at $T < T_c$[3,4]. This sharp change in the type and density of the dominant charge carriers is naturally explained by the restructuring of the bands that takes place as a result of the excitonic instability[5], and further reinforces the key role that this mechanism plays in the CDW transition of $TiSe_2$.

### S-I.D. Validity of the single valence band approximation

When in the main text we introduced the effective parameterization of the electron and hole pockets for the self-consistent calculation of the excitonic instability, we noted that, although DFT calculations yield two valence bands crossing $E_F$ near the $\Gamma$ point, in our studies, we modeled the system with only one. This has also been the approach consistently followed in the literature of this system[5–7]. There are good reasons for such a simplified treatment:

First, the size of the pockets arising from the DFT calculation is strongly sensitive to the functionals and refinements beyond the Local-density approximations. This is not surprising given the extremely reduced carrier density of the system and the known issues with DFT implementations

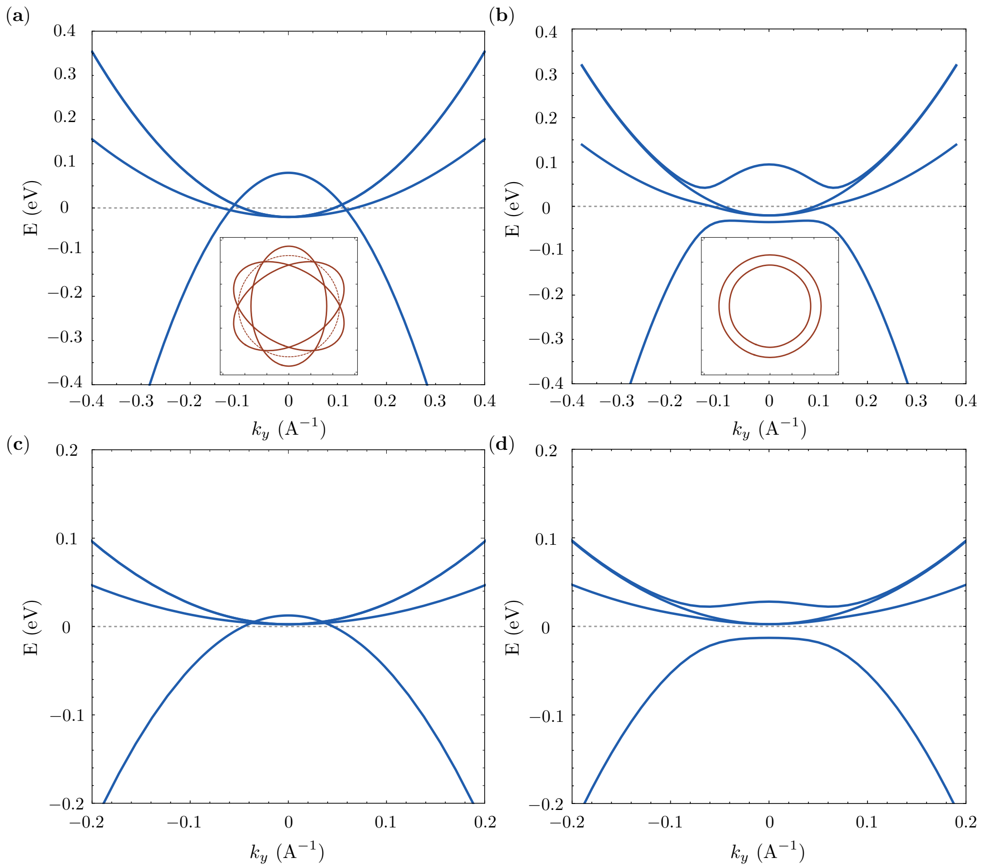


FIG. S3. Bare and renormalized (folded) bandstructure in the excitonic phase. (a) and (b) show, respectively, the bare and the renormalized bands for $\epsilon_{bo} = 0.1$ eV. The insets show the corresponding Fermi surfaces with the dashed circle marking the hole pocket. (c) and (d) show the equivalent representation at $\epsilon_{bo} = 0.01$ eV. The curves are plotted in the reduced Brillouin zone as a function of $k_y$ near the folded Γ point. The chemical potential ($\mu$, dashed gray line at $E = 0$) is set at the value that corresponds to the highest transition temperature for each case (see Fig. 3 in the main text).

capturing band gaps with quantitative accuracy. A reflection of the typical "gap underestimation problem" in our GGA calculation is that the valence bands lie too high in energy, thus leading to large hole pockets. In fact, supplementary supplementary Fig. S6 shows that there is a considerable difference when the calculation is done at the HSE06 level (which counteracts the underestimation): in this case the splitting between the two valence bands is larger and only one hole pocket arises. In addition to this, there is the critical aspect we point out in our discussion and interpretation that the DFT calculation cannot capture the excitonic effects anyway. Therefore, from a DFT point of view it is not clear at the current stage (from our calculations and all those we are aware in the literature) what the accurate "reference" bandstructure is in the normal state, namely whether

there are two or one electron pockets. Hence, there is no basis in using the DFT results of Fig. 3 to conclude that, in order to capture the real situation, one must explicitly include the two valence bands in the mean-field calculation.

Secondly, from the experimental point of view, unfortunately, the situation cannot be unequivocally clarified either because of the extremely small carrier densities that prevent clear access to the conduction bands in ARPES, or because of the above-mentioned fact that CDW/excitonic fluctuations likely cause the system to appear with reconstructed/hybridized bands above the mean-field $T_c$. Actually, this has been one of the key challenges in settling the nature of the CDW instability in this system because, despite the ability to obtain good-resolution ARPES data, their interpretation has been made in opposing ways through the years in the literature.

Finally, the ARPES data and DFT-HSE calculations reported by Chen et al.[8] (Fig. 2a in that paper) do show that the separation of the two valence bands is approximately well captured by the HSE calculation (but not their absolute position, which must be rigidly shifted as the authors state, nor the relative position with respect to the conduction bands). This makes it likely that the normal state has only one hole pocket, which would be also consistent with the fact that this second valence band is much less sensitive to temperature, as can be seen in Fig. 3 of the same reference. At any rate, since in the experiments the two bands are distanced by $\approx 0.2$ eV, one expects the effect of a putative second pocket, if it exists, to be a correction to the dominant hybridization taking place in the valence band closest to $E_F$. From the point of view of our mean field calculation, it is not unreasonable to admit that such a correction due to an additional hole pocket could be absorbed in a new value of the interaction parameter of the theory (i.e., in practice treating the two hole pockets as an "effective" single one). For this reason, we do not anticipate different results (neither qualitatively nor quantitatively) if our self-consistent calculation were to be carried out with two hole pockets from the outset.

### S-I.E. Mapping chemical potential to doping introduced by Cu intercalation

Our calculations of the excitonic instability are performed at constant chemical potential ($\mu$) which, together with the temperature ($T$), constitute our externally set thermodynamic parameters. The phase diagram shown in Fig. 1 of the main text is drawn in terms of these two parameters. In order to compare the suppression of critical temperature ($T_c$) predicted by the excitonic instability with the experimental data available for Cu-intercalated $TiSe_2$, the chemical potential was mapped to the Cu content ($x$) in $Cu_xTiSe_2$ as follows.

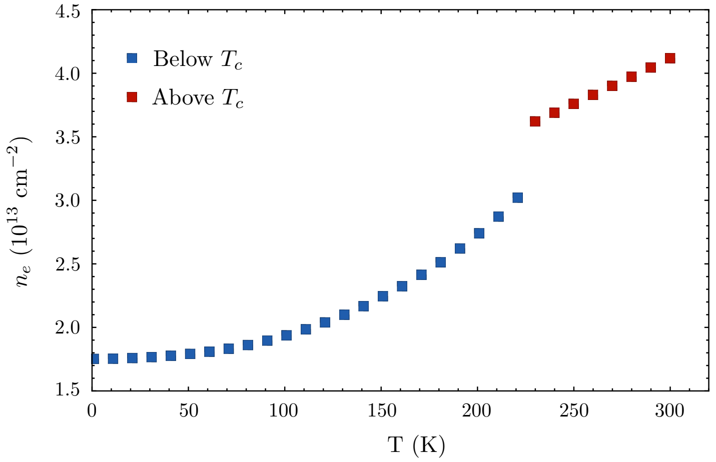


FIG. S4. The electron density above and below $T_c$ at zero doping ($x = 0$). The chemical potential is set as in Fig. S3(a) and we used $\epsilon_{bo} = 0.1$ eV.

Since each Cu atom contributes one additional electron to the system, in $Cu_xTiSe_2$ there will be $x$ additional electrons in each unit cell. Thus the increase of electronic density would be $x/\Omega$, where $\Omega$ stands for the area of the unit cell. When the chemical potential $\mu$ is increased with respect to its pristine value ($\mu_0$), the electron (hole) density in the conduction (valence) bands will increase (decrease). Defining $\Delta n_e(\mu) \equiv n_e(\mu) - n_e(\mu_0)$ and $\Delta n_h(\mu) \equiv n_h(\mu) - n_h(\mu_0)$ to denote them separately, charge conservation implies

$$\Delta n_e(\mu) - \Delta n_h(\mu) = x/\Omega, \tag{S9}$$

where the left-hand side of Eq. (S9) can be directly calculated from the electronic band structure.

As an illustration, Fig. S4 shows the electronic density at different temperature and $x = 0$, holding the chemical potential fixed as in Figs. S3(a). The strong drop at $T_c$ is related, primarily, to the partial removal of electron states in the CDW phase and, in addition, to the reconstructed bandstructure whose changes have the most impact for small doping [cf. Fig. S3(b)]. This must have a direct and strong impact in electronic transport by an increase in the resistance. Experimentally, $TiSe_2$ samples consistently exhibit a characteristic and marked upturn in longitudinal resistivity that accompanies the CDW transition in $TiSe_2$. This transport signature has been experimentally observed since the early experiments[3] and the sudden increase registered in $\rho(T)$ around $T_c$ is frequently used to track $T_c$ as a function of other experimental parameters[2,4]. According to the excitonic mechanism, in addition to contributions from scattering by CDW fluctuations in the vicinity of $T_c$, that signature might be also directly related to the suppression of electronic states as the transition takes place.

# S-II. ELECTRON-PHONON COUPLING AND ELECTRON-ELECTRON INTERACTION

In the main text, we have taken into account the electron-electron interaction and studied the excitonic condensation. However, due to the formalism of mean-field theory, one might realize that an same approach to a Hamiltonian with *only* electron-phonon coupling will lead to a same type of gap equation as we had before. In fact, there have been works where both kind of effects were considered[7,9–11], however, they are either not fully self-consistent[7,9] or were done on an simplified (quasi-1D) version of the Hamiltonian[10,11]. A fully self-consistent study based on the exact Hamiltonian is needed.

In this section, we will show that, even in a system with both electron-electron interaction and electron-phonon coupling, the final form of the gap equation for the charge density order parameter will be similar to the one we have in Eq. (S8).

## S-II.A. Mean-field description of the CDW with both excitons and phonons

One should point out that the self-consistent equations that arise from the mean-field decoupling in (S3) and (S4) would be formally equivalent if, instead of through Coulomb interaction, the electron-hole pockets in the original Hamiltonian are coupled by phonons in the way of Fröhlich[12] at $\mathbf{Q}_{\text{cdw}}$. In order to consider both types of interaction, one just needs to add the free phonon part and the electron-phonon coupling to the Hamiltonian we have considered in the main text. A similar type of treatment has also been implemented by B. Zenker et al. in studying the chiral CDW phase[13]. Supposing the electron-phonon coupling is of the form:

$$H_{\text{e-p}} = \frac{1}{\sqrt{N}} \sum_{i} \sum_{\boldsymbol{k},\boldsymbol{q}} g_{\boldsymbol{k},\boldsymbol{Q}_i+q} d^{\dagger}_{i,\boldsymbol{k}+\boldsymbol{q}} c_{\boldsymbol{k}} \left( a_{\boldsymbol{Q}_i+\boldsymbol{q}} + a^{\dagger}_{-\boldsymbol{Q}_i-\boldsymbol{q}} \right) + \text{h.c}, \tag{S10}$$

the mean field Hamiltonian would be of the form

$$H = H_1 + H_2 \tag{S11}$$

$$H_1 = \sum_{\boldsymbol{q}} \hbar\omega_{\boldsymbol{q}} a^{\dagger}_{\boldsymbol{q}} a_{\boldsymbol{q}} + \sqrt{\frac{1}{\mathcal{N}}} \sum_{i,\boldsymbol{k}} g_{\boldsymbol{k},\boldsymbol{Q}_i} \left[ \left\langle d^{\dagger}_{i,\boldsymbol{k}} c_{\boldsymbol{k}} \right\rangle \left( a_{\boldsymbol{Q}_i} + a^{\dagger}_{-\boldsymbol{Q}_i} \right) + \left\langle c^{\dagger}_{\boldsymbol{k}} d_{i,\boldsymbol{k}} \right\rangle \left( a^{\dagger}_{\boldsymbol{Q}_i} + a_{-\boldsymbol{Q}_i} \right) \right] \tag{S12}$$

$$H_2 = \sum_{\boldsymbol{k},\sigma,i} \varepsilon_{v\boldsymbol{k}} c^{\dagger}_{\boldsymbol{k},\sigma} c_{\boldsymbol{k},\sigma} + \varepsilon_{\boldsymbol{k},i} d^{\dagger}_{i,\boldsymbol{k},\sigma} d_{i,\boldsymbol{k},\sigma} - \sum_{\boldsymbol{k},\sigma,i} \left( \Delta_{i,\boldsymbol{k},\sigma} + \delta_i \right) c^{\dagger}_{\boldsymbol{k},\sigma} d_{i,\boldsymbol{k},\sigma} - \left( \Delta^{*}_{i,\boldsymbol{k},\sigma} + \delta_i \right) d^{\dagger}_{i,\boldsymbol{k},\sigma} c_{\boldsymbol{k},\sigma}. \tag{S13}$$

Assuming the order parameters are real and do not depend on the direction of the CDW and momentum $\boldsymbol{k}$, we have the following expressions for both order parameters:

$$\Delta \equiv \frac{1}{\mathcal{N}} \sum_{k} V \left\langle d_{i,\boldsymbol{k}}^{\dagger} c_{\boldsymbol{k}} \right\rangle , \tag{S14}$$

$$\delta_i = -\frac{1}{\sqrt{\mathcal{N}}} g \left\langle a_{\boldsymbol{Q}}^{\dagger} + a_{-\boldsymbol{Q}} \right\rangle = \frac{1}{\mathcal{N}} \frac{g^2}{\omega_{\boldsymbol{Q}}} \sum_{\boldsymbol{k}} \left( \left\langle c_{\boldsymbol{k}}^{\dagger} d_{i,\boldsymbol{k}} \right\rangle + \left\langle d_{i,\boldsymbol{k}}^{\dagger} c_{\boldsymbol{k}} \right\rangle \right) = 2 \frac{g^2}{\omega_{\boldsymbol{Q}} V} \Delta. \tag{S15}$$

If one compares $H_2$ and the mean field Hamiltonian in equation (4) of the main text, it can be easily seen that, now, the term $\left(1 + 2g^2/\omega_{\boldsymbol{Q}} V\right) \Delta_i$ plays the role of $\Delta_i$ before. It is also important to notice that the *plus* sign here indicates that both interactions collaborate to the CDW transition. One can show that the gap equation for $\Delta_i$ is of a similar form to the one discussed in the main text, namely:

$$\Delta + \frac{k_B T}{\mathcal{N}} \sum_{k,\omega_n} \frac{AV \left(1 + \frac{2g^2}{\omega_{\boldsymbol{Q}} V}\right) \Delta}{\left(1 + \frac{2g^2}{\omega_{\boldsymbol{Q}} V}\right)^2 \Delta^2 B - C} = 0, \tag{S16}$$

with the definitions $\alpha = 1 + 2g^2/\omega_{\boldsymbol{Q}} V$, $V' = \alpha V$ and $\Delta' = \alpha \Delta$. The gap equation above can be recast as

$$\Delta' + \frac{k_B T}{\mathcal{N}} \sum_{k,\omega_n} \frac{AV'\Delta'}{\Delta'^2 B - C} = 0, \tag{S17}$$

which is exactly the same as equation (9) with the following identifications:

$$V' \leftrightarrow V, \qquad \Delta' \leftrightarrow \Delta. \tag{S18}$$

Because of the simple linear relationship between $V, \Delta$ and $V', \Delta'$, the solution of Eq. (S17) gives rise to a unique solution for $\Delta$. Correspondingly, the transition temperature is also the same in both cases if $V'$ here is equal to the value of $V$ in the main text.

Consequently, equation (S8) is formally unchanged if one considers both excitons and electron-phonon coupling at $\boldsymbol{q} = \mathbf{Q}_{\mathrm{cdw}}$ from the outset, in which case $V$ and $\Delta$ are reinterpreted in terms of the combined parameters. But, on the one hand, doing so increases the number of parameters in the theory, which might seem unnecessary since it has been previously shown that, if the excitonic mechanism alone can capture the experimental temperature dependence, the lattice responds with a PLD in agreement with experiments[7]. On the other hand, one anticipates a dominant effect of the electronic interactions because of the very small carrier densities. This suggests that, despite the fact that both phonons and excitons will necessarily be coupled and soften together, one should

assign a strong excitonic character to this instability. Finally, a full self-consistent treatment of both mechanisms would always be limited by the inability of accurately describing the phonon spectrum as a function of temperature. Instead, we corroborate the importance of interactions by determining the predictions that follow in their absence using unbiased, state of the art DFT computations of the phonon instabilities and bandstructures of $TiSe_2$ with doping. Since these, predominantly accounting for the electron-phonon coupling, fail to accurately describe the doping dependence, we conclude that the relative contribution of the excitons to the mean field phase diagram cannot be small, and is likely to be dominant.

### S-II.B. Estimating the lattice distortion in the excitonic-condensed state

Monney *et al.* have recently shown that, given a finite order parameter $\Delta(T)$ whose temperature dependence follows the experiments, combining the exciton condensate with electron-phonon coupling leads to a PLD with correct order of magnitude in the lattice displacement of undoped $TiSe_2$[7]. Although their calculation is not self-consistent and only establishes how the lattice softens in response to the exciton condensate, the result does reinforce the strong influence that the excitonic instability can have in the stability of the lattice.

Furthermore, incorporating our self-consistent calculation of $\Delta$ in the $(T, x)$ parameter space (Fig. S2) into such calculations, provides a complete picture of the CDW/PLD in $TiSe_2$ with electronic and lattice degrees of freedom. This would not be surprising in itself because electronic interactions are known to be sufficient to stabilize robust CDW phases even in the absence of a PLD, particularly in reduced dimensions[14–18]. However, it would be incorrect to consider phonons as simple spectators because, on the one hand, self-consistency involving both electron-electron and electron-phonon interaction is expected to further stabilize the PLD; on the other hand, the latest experimental evidence shows that this system carries hybrid electronic and lattice elementary excitations close to $T_c$[19].

## S-III. THE LATTICE INSTABILITY *AB-INITIO*

### S-III.A. Details of the DFT calculations

Our *ab initio* calculations were done within the DFT framework[20] with the projector augmented wave method implemented in the Vienna Ab-initio Simulation Package (VASP)[21,22]. Except when stated otherwise, we resort to the generalized gradient approximation (GGA)[23] for the exchange-

correlation functional and include spin-orbit coupling. To simulate the normal and distorted $TiSe_2$ monolayers, a thick vacuum slab of more than 12 Å is used to prevent interaction between the periodically repeated images. The BZ was sampled with a Γ-centered $16 \times 16 \times 1$ $\boldsymbol{k}$-mesh and a plane wave basis set with energy cut-off of 380 eV. The in-plane lattice constant and atomic positions were relaxed until residual forces became less than 1 meV/Å. Force constants were obtained within density functional perturbation theory (DFPT) and the phonon dispersions computed with the PHONOPY code[24,25].

Ground-state electronic and vibrational properties are calculated with a small smearing parameter ($\sigma = 0.01$ eV). Technically, this is a parameter to accelerate convergence without direct physical meaning; it acquires the physical meaning of electronic temperature only when used in conjunction with finite temperature smearing methods[26–28]. We discuss results obtained with different smearing strategies in one of the supplementary sections further down.

In order to facilitate a direct comparison of calculated energy spectra with the available ARPES results, we perform the unfolding of the supercell band structure to the primitive cell BZ. The essence of this procedure is to find a plane wave in the supercell BZ associated with a primitive cell's $k$-point. This is done by projecting the supercell wavefunctions onto primitive cell and calculating spectral weights as discussed in references 28 and 29.

The effects of additional carriers in $TiSe_2$ were investigated with two complementary strategies. First, we explicitly studied the doping induced by Cu by simulating supercells with adsorbed Cu. Subsequently, for the systematic study of the phonon instabilities, electron (hole) doping was considered by adding (removing) electrons to the unit cell, with a neutralizing uniform background charge.

The internal atomic positions in the unit cell were relaxed for each doping while keeping the lattice parameter fixed at its undoped value. For the study of Cu-intercalated $TiSe_2$, Cu atoms were placed directly above and below the central Ti in a $2 \times 2$ supercell [see Figs. S1 (a)-(b)]. All the atoms were allowed to freely relax inside the unit cell. Interestingly, despite unconstrained, the Cu atoms adsorb onto the surface without bouncing back into the vacuum with an adsorption energy of $E_{ads} = 2.456$ eV/Cu, where $E_{ads} = -[E_{rel}(\mathrm{Cu}_x\mathrm{TiSe}_2) - E_{rel}(\mathrm{TiSe}_2) - E(\mathrm{Cu})]$. The structural stability of these Cu-adsorbed $TiSe_2$ monolayers was further scrutinized by calculating the phonon spectrum.

To track the evolution of $\sigma_c$ with electron density, we calculated the phonon spectrum covering a range of different $\sigma$ for each doping. Fig. S9(a) shows the representative case of $x = 0.04$ where the imaginary frequencies disappear if $\sigma > 0.4$ eV. As this threshold smearing is very similar to that

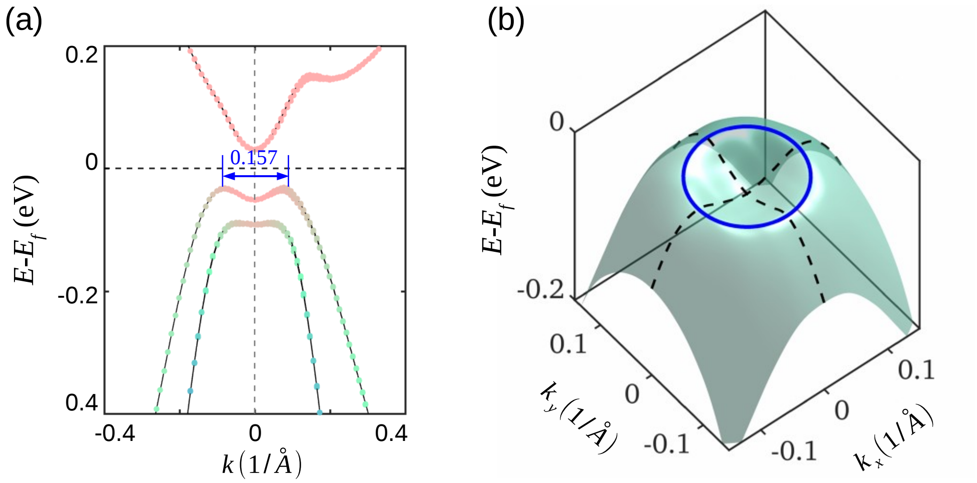


FIG. S5. (a) Electronic band structure of undoped $TiSe_2$ monolayers with the PLD. (b) Zoom-in structure of top valence band in the $E - k_x - k_y$ space within the reduced Brillouin zone. Black dashed lines show the band structure along two orthogonal directions and blue ring highlights the valence band maximum in the reduced Brillouin zone.

of the undoped monolayer, it would suggest that the CDW/PLD phase is as robust at this doping as in pristine form, unlike the experimental situation!

### S-III.B. Renormalized band structure: Mexican hat features

In Fig. S5 we show a close-up of the restructured bands in undoped $TiSe_2$, whose ground state we determine to be the $2 \times 2$ PLD with wavevector $\mathbf{Q}_{\mathrm{cdw}}$ after full relaxation of the ions in the unit cell [see also Fig. 3 in the main text]. The top valence bands are seen to lose their $-k^2$ parabolic dispersion and develop the shape of an inverted Mexican hat. More specifically, the top of the valence band moves from $k = 0\,\text{Å}^{-1}$ to lie at $k = 0.0785\,\text{Å}^{-1}$. A 3D rendition of this band shows that the maximum defines a circle of diameter $0.157\,\text{Å}^{-1}$ centered at $k = 0$, as marked by the blue circle in Fig. S5. This is additionally supported by the fact that the energy dispersion along two orthogonal directions flattens exactly on this circle. Both perspectives establish the inverted Mexican hat shape of the band dispersion in the distorted phase (ground state). As discussed earlier by Kohn[30] and emphasized by Cazzaniga *et al.* with DFT+GW calculations for bulk $TiSe_2$[31], this shape is typical of the excitonic phases.

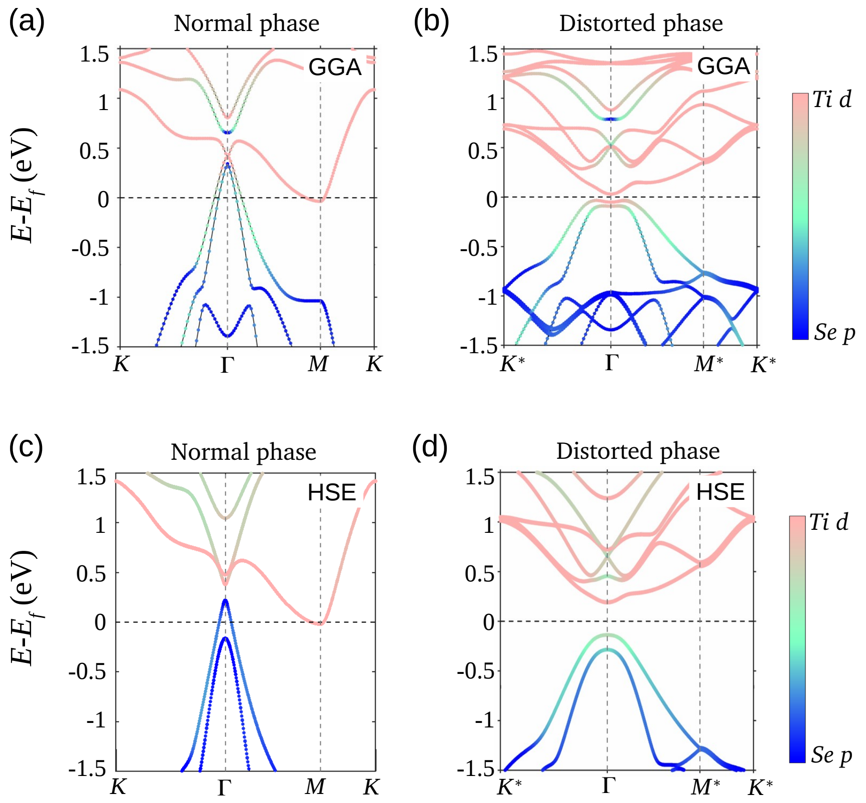


FIG. S6. Electronic band structure of the (a,c) normal and (b,d) distorted phase of undoped $TiSe_2$ calculated with GGA (top row) and HSE (bottom row). The semimetal nature of the normal phase and the gapped state of the distorted one remain robust with these functionals.

### S-III.C. GGA and HSE band structure of normal and distorted phase

Local and semi-local GGA functionals normally underestimate the orbital occupations. The more advanced HSE exchange-correlation functional uses a part of exact Fock exchange and is known to correct the orbital occupations, yielding results in closer agreement with experimental band structures. We computed the band structure of the normal and distorted phases using the GGA and the HSE06[32] hybrid.

In Fig. S6, we compare the band structures of the normal and distorted phases of monolayer $TiSe_2$ obtained with these two energy functionals [the GGA band structures shown in Figs. S6(a)-(b) are also presented in the main text in Figs. 3(a) and 3(c)]. As discussed in the main text, the normal phase GGA band structure has a semimetal character with a clear energy overlap between the valence and conduction states. The HSE band structure, on the other hand, shows a rigid shift of the valence and conduction states with a decrease in the band overlap, Fig. S6(c), but still retaining the semimetal character in the normal phase.

In the distorted phase, the HSE band structure shown in Fig. S6(d) retains the overall features of the bands in the GGA, including the semiconducting (gapped) state. However, the hybridization of the valence and conduction bands leads to an energy gap of 325 meV which considerably overestimates (by 172 meV) the experimentally reported value of $\simeq 153$ meV (at 10 K)[8,28]. By comparison, the GGA gap is $E_{\rm g} = 82$ meV, which underestimates the experimental value by 71 meV. An underestimation of the calculated gap is generically expected in the absence of quasiparticle (GW) corrections. In addition, the inverted Mexican hat profile of the valence states is nearly suppressed in the HSE result: the diameter of the Mexican hat is much smaller than in the GGA (Fig. S5) to the extent that, while it is clearly visible in Fig. S6(b), it is not resolved in the equivalent plot of Fig. S6(d).

The larger deviation (and overestimation) of the band gap and the near suppression of the band restructuring near $E_F$ within HSE, justifies our choice of using the GGA to compute the band structure of both electrons and phonons in this problem.

### S-III.D. Unfolded bands with and without doping or distortion

In Fig. S7 we reproduce the band structures shown in Fig. 3 of the main text. As described there, these were obtained using a $2 \times 2$ unit cell. Panel (a) shows the resulting dispersion when the ions are held in place; it simply corresponds to the band structure of the normal (undistorted) phase in the reduced Brillouin zone identified by the dashed honeycomb in Fig. S1(c). Panel (b) shows the electronic spectral function of the same bands unfolded back to the original ($1 \times 1$) Brillouin zone, where one sees the familiar hole pocket at $\Gamma$ and the electron pocket(s) at $M$.

Fig. S7(c) shows the band structure generated when the ions are allowed to relax freely within the $2 \times 2$ unit cell: The system reaches the ground state by creating a lattice distortion which, simultaneously, reshapes the bands near $E_{\rm F}$ as discussed earlier and lowers the total energy. The corresponding spectral function in the unfolded zone is plotted in panel (d). In contrast with (b), we now see spectral weight that duplicates the hole dispersion originally near $\Gamma$ around $M$, and electron dispersion originally around $M$ gets shadowed around $\Gamma$. This agrees with ARPES measurements in both bulk[6] and monolayer samples[8].

Fig. S7(f) shows the unfolded spectral function associated with the bands in panel (e). It illustrates that, just as doping has little effect in the band structure near the pocket intersection, doping has also a mild effect in the shadowing of spectral weight. Note that, as explained in the main text, the band structures shown in (e,f) have been obtained with two relaxed Cu atoms in the

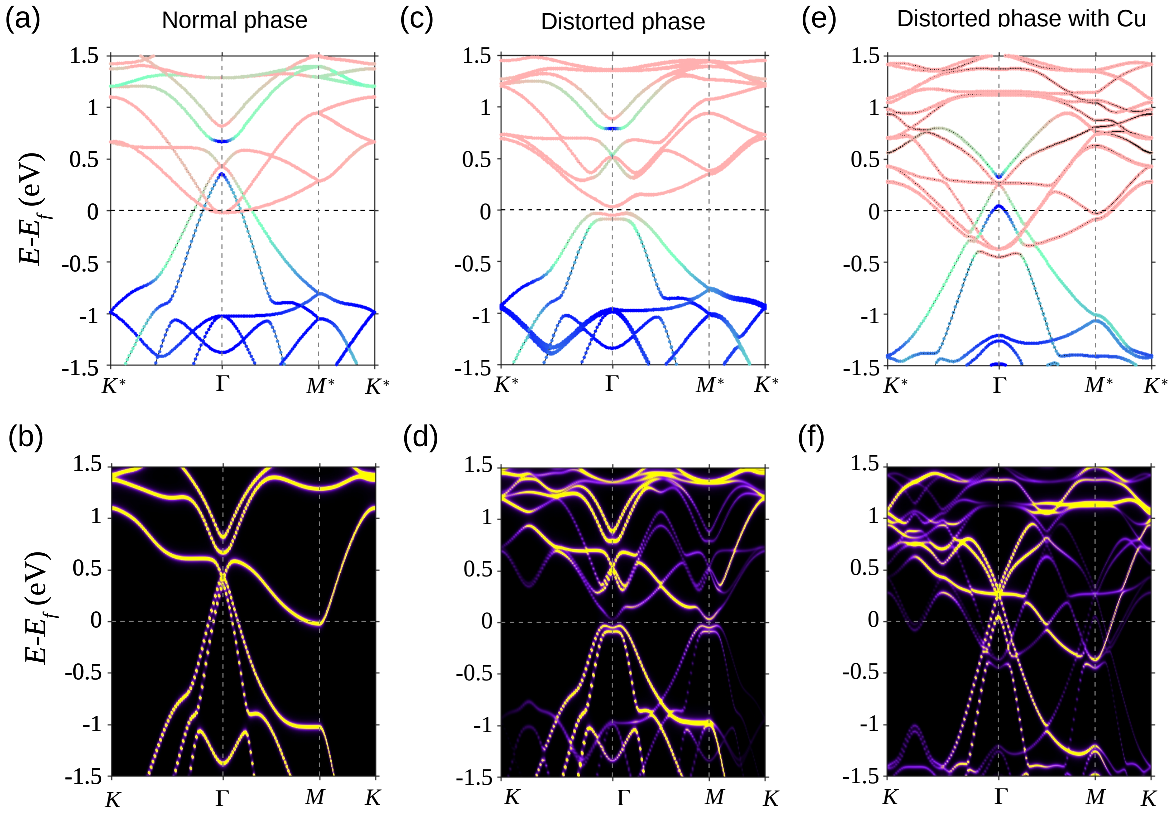


FIG. S7. Effect of the PLD and Cu doping on the electronic structure of $TiSe_2$. Shown are the band structure in the unrelaxed, normal phase (a,b), in the relaxed distorted phase (c,d), and in the relaxed phase with Cu doping (e,f). Each column plots the bands in the $2 \times 2$ reduced Brillouin zone of the distorted phase (top) and the corresponding unfolded version in the BZ of the undistorted phase (bottom). The bands obtained without lattice relaxation in (a) have the Ti-derived electron pocket folded into the Γ point without any restructuring or gap opening; they are restored back to the $M$ point in the unfolded representation (b). The situation is quite different when the lattice is allowed to relax on a $2 \times 2$ supercell: in addition to the spontaneous lattice distortion, we observe a finite band gap and the appearance of two back-folded bands at the M point (c,d). Adsorbed Cu atoms electronically dope the system and raise the Fermi level higher in the conduction bands without noticeable disruption to the overall dispersion (e,f) in comparison with the undoped case (c,d).

$2 \times 2$ unit cell, thus corresponding to a Cu:Ti ratio of 50%. This is extremely high, in comparison with the experimental solubility limit of 11%[4,33]. Yet, the main effect is electron doping without significant qualitative change in the energy band dispersion.

### S-III.E. Effective mass from ARPES and DFT calculations

As described in the main text, our calculations of the excitonic instability rely entirely on the bandstructure parameters obtained from ARPES in the normal state, which are stated in footnote/reference [39] of the manuscript. The effective masses, in particular, are $m_{c,\|} = 3.46 m_e$, $m_{c,\perp} = 1.38 m_e$, $m_v = 0.63 m_e$. From our DFT GGA calculation we obtain $m_{c,\|} = 3.46 m_e$ and $m_{c,\perp} = 0.22 m_e$. On the other hand, the relevant valence band obtained from DFT deviates quickly from a quadratic dispersion (hyperbolic like); the best approximation to a quadratic dispersion yields about $m^v_{\text{DFT}} \sim 0.19 m_e$.

As far as the CDW instability is concerned, the most relevant comparison is expected to be for the effective masses along the direction of $\mathbf{Q}_{\text{cdw}}$ (i.e., the $m_\|$). In the conduction band, the ARPES-derived and DFT-calculated $m_\|$ match well. The mass associated with the (isotropic) valence band is however off by a factor of about 3. But, even though one could suggest that, by predicting the valence electrons to be too light, DFT is missing effects of quasiparticle mass renormalization due to interactions that are either missed or incompletely taken into account, such statement cannot generally be put on solid ground: on the one hand, the GGA framework always treats the correlation problem in an effective way, preventing a direct quantitative assessment of these effects; on the other hand, such comparison is looking at the effective masses in the normal/undistorted phase which is not the true ground state of the lattice. In other words, we can conceive a situation in which, despite moderate interactions, the band parameters for the true ground state are in acceptable agreement, but forcing a DFT bandstructure calculation in the $1 \times 1$ state might yield a large discrepancy in comparison with the experimental spectral function obtained in the normal state.

### S-III.F. Phonon hardening with Cu doping

As discussed in the main text as well in our earlier work[28], the low-temperature state of an undoped $TiSe_2$ monolayer is the CDW phase with an accompanying PLD. Our DFT and DFPT calculations demonstrate that Cu adsorption (which corresponds to intercalation in bulk systems) suppresses the PLD and eventually stabilizes a $1 \times 1$ undistorted structure at zero temperature. In the main text, this transition as a function of doping is established by studying the density beyond which the dynamical phonon instability disappears at $T = 0$ (cf. Fig. 4); as explained and justified there, these calculations are done by adding additional electrons to the unit cell.

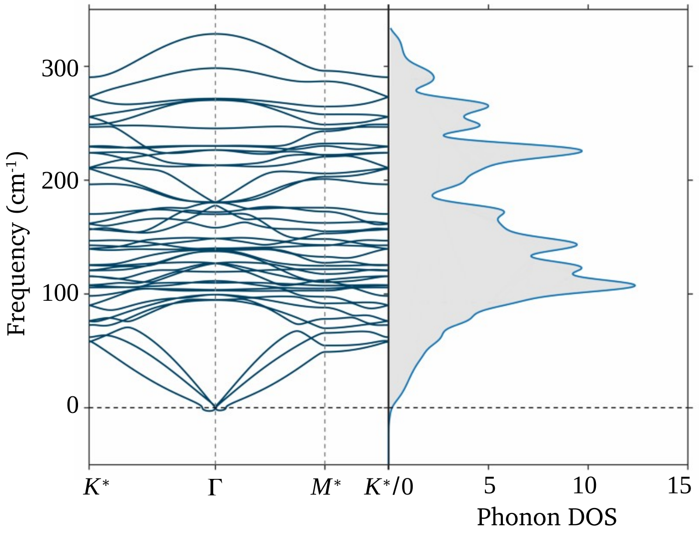


FIG. S8. Phonon band dispersion (left) and phonon density of states (right) of a Cu-doped $2 \times 2$ $TiSe_2$ monolayer at low smearing parameter. The absence of imaginary frequencies in the reduced Brillouin zone confirms the dynamical stability in the presence of the Cu adsorbates.

Here, we wish to demonstrate that this conclusion holds when the phonon spectrum is computed including the Cu atoms explicitly in the unit cell from the outset. Fig. S8 summarizes the phonon spectrum and corresponding density of states obtained under such conditions, with two Cu atoms per $2 \times 2$ supercell (one adsorbed above and the other symmetrically below the $TiSe_2$ monolayer, as in Fig. S1(b)). We highlight that this phonon spectrum has been calculated using the same structure that is employed to determine the band structure shown in Fig. 3(c) of the main text. Fig. S8 does not show any imaginary frequencies nor soft acoustic branch, thereby confirming the dynamical stability of the Cu doped monolayer at low temperature. This small simulation cell corresponds to a 50 % Cu content ($x = 0.5$), it tallies with the evolution of $\sigma_c$ shown in Figs. 1 and 4 (main text) based on the electron doping approach that predicts the lattice to be stable for $x \gtrsim 0.20$. It also reinforces the validity of the latter approach for numerical expediency in treating the experimentally relevant doping levels of $0 < x < 11$ which, to explore with actual Cu atoms in the supercell, would require extremely large supercells, prohibitive for both the DFT electronic structure and DFPT phonon calculations.

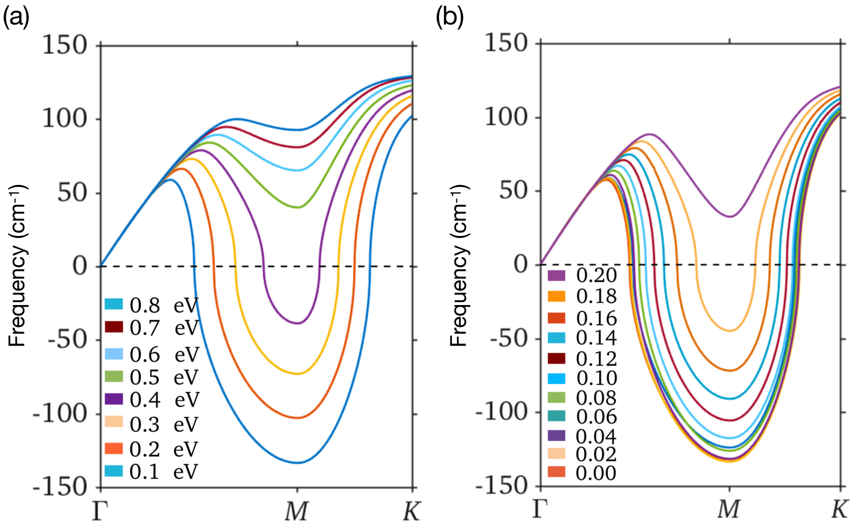


FIG. S9. Calculated phonon modes and the suppression of the PLD in the $TiSe_2$ monolayer with temperature and doping. (a) The soft mode along the relevant high-symmetry directions for different $\sigma$ (see legends) and fixed doping of $x = 0.04$ electrons per formula unit (e/fu). (b) Same as (a) but for different electronic doping at fixed $\sigma = 0.01$ eV. Legends show $x$ in e/fu.

### S-III.G. Robustness of the PLD and CDW transition with smearing function

In electronic structure calculations, the smearing function is routinely used to decide how to set the partial occupancies for each wavefunction. For a particular smearing method, $\sigma$ determines the width of smearing. An optimal choice for smearing function and $\sigma$ depends not only on improved convergence but also on the system and properties of interest. However, all methods should converge to the ground state in the limit $\sigma \to 0$.

In order to verify the robustness of our conclusions regarding the evolution of the dynamical phonon instability and PLD with doping, we calculated the phonon dispersions of undoped $TiSe_2$ using two independent strategies: the Mehfessel-Paxton (MP) smearing and Fermi-Dirac (FD) smearing methods. The resulting phonon spectra at different $\sigma$ are shown in Fig. S10. It is evident that both approaches correctly predict the freezing of the longitudinal acoustic mode at the experimentally correct $\mathbf{Q}_{\rm cdw}$, and the existence of a threshold $\sigma_c$ above which this instability suppressed. Note, however, that the magnitude of $\sigma_c$ varies for different smearing strategies, and reflects the fact that $\sigma$ is not the physical temperature, and should only be used to explain qualitative trends in the lattice structure as a function of temperature. These results are consistent with earlier calculations done for bulk $TiSe_2$[27].

One of our central conclusions in the main text is that relying only on the phonons calculated

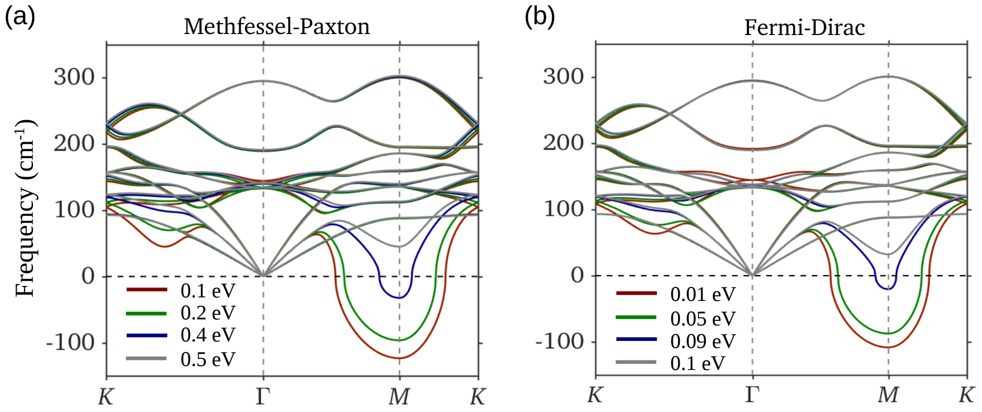


FIG. S10. Phonon dispersion of the $1\times1$ $TiSe_2$ monolayer (normal phase) calculated with different smearing parameter ($\sigma$) using: (a) Metthfessel-Paxton smearing and (b) Fermi-Dirac smearing. Imaginary frequencies are represented as negative values.

within DFT+DFPT to predict the critical doping ($x_c$) above which the CDW/PLD is no longer stable, leads us to values of $x_c$ that overshoot the experimental threshold by about one order of magnitude. Crucially, this result is also independent of the smearing method used, as we show in Fig. S11: both MP and FD smearing predict the PLD to remain as the ground state at least up to $x = 0.16$. Conversely, this implies, by extrapolation, that $x_c \gtrsim 0.20$ if $x_c$ is extracted from the criterion $\sigma_c(x) = 0$.

Seeing that there is complete consistency among the calculated phonon dispersion and phonon instabilities with these two smearing methods, we chose to present in the main text the results obtained with the Mehfessel-Paxton smearing because of its improved convergence and accuracy over Fermi-Dirac smearing.

It is important to remark, though, that the actual relation between $\sigma$ and $T$ depends on the smearing strategy used. In addition, the physical temperature includes contributions not only from the electrons but also from the phonons. However, although this means that $\sigma_c$ cannot be directly related to $T_\mathrm{c}$, existence of a finite $\sigma_c$ can be safely used to predict a finite $T_\mathrm{c}$.

## S-IV. PERTINENCE OF STUDYING A MONOLAYER FOR THE BULK SYSTEM

We studied the monolayer $TiSe_2$ in the mean field calculation and compared the results with existing experiments on bulk systems. As a matter of principle, quantum confinement effects can lead to quantitative and/or qualitative differences in the electronic band structures of monolayer and bulk $TiSe_2$. However, as discussed in various previous studies, as well as reported in recent

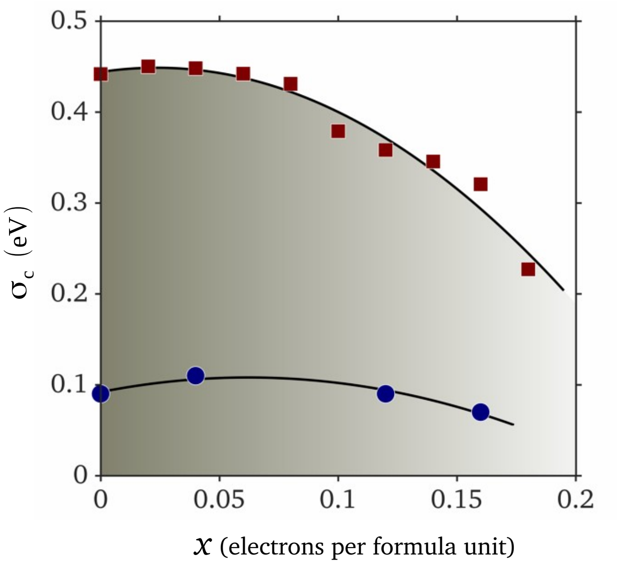


FIG. S11. The critical smearing parameter ($\sigma_c$) as a function of doping $x$ according to the two different smearing strategies discussed in the text. The values of $\sigma_c$ are obtained from studying the phonon spectrum for different $\sigma$ as in Fig. S10. All phonon frequencies are real (no dynamical instability) for $\sigma > \sigma_c$. The red points were obtained with Metthfessel-Paxton and the blue using Fermi-Dirac smearing (black lines are guides). Note how, despite having different magnitudes (see text), the two strategies agree in the qualitative prediction that the phonon instability persists up to very large values of $x$.

experiments, the CDW transition in both monolayer and bulk $TiSe_2$ involves the interplay of states that lie within a narrow energy of $E_F$. These states are represented by the Se $p$-derived top portion of the highest valence band and Ti $d$-derived bottom portion of the lowest conduction band. Other bands located elsewhere in the Brillouin zone near the Fermi level are insensitive to the atomic distortion associated with the CDW transition and do not contribute significantly to the energetics and stability of the CDW in either bulk or monolayer $TiSe_2$[5,8,28,31].

The observed experimental spectral function in the normal and CDW phases of the monolayer clearly resembles the spectral function of the bulk. Furthermore, it has been established experimentally that the evolution of the CDW phase with carrier density, as well as the onset and shape of the superconducting dome, is qualitatively and quantitatively similar in atomically-thin films and bulk samples[2,4]. This clearly indicates that the CDW physics in monolayer $TiSe_2$ is similar to that of the bulk, and that intra-layer electronic and phononic processes are clearly dominant in determining the phase transitions. This, of course, is not surprising given the strongly two-dimensional character (both structurally and electronically) of the bulk crystal, imposed by the vertical stacking of weakly coupled $TiSe_2$ monolayers.

It should be noted that despite decades of experimental and theoretical studies on bulk $TiSe_2$, the CDW physics in this system remains controversial. Obvious reasons involve the 3D nature of the CDW order in bulk crystals, which challenges the identification of the exact gap locations and weight transfer in the 3D Brillouin zone. As demonstrated by recent experiments on monolayer[8,34] and thin films[2,35], individual layers of $TiSe_2$ undergo a $2 \times 2$ transition at temperatures close to those of the bulk $T_c$ (slightly higher due to reduced screening, see below), with density modulation of wavevector $\mathbf{Q}_{\rm cdw} = \Gamma M$. This $\mathbf{Q}_{\rm cdw} = \Gamma M$ in the monolayer system corresponds precisely to the projection of the three-dimensional wavevector ($\Gamma L$) onto the horizontal plane[3]. The difference between the charge-density profile in individual layers and bulk is that, in the latter, the Van der Waals stacking in the third dimension causes neighboring layers to lock their individual $2 \times 2$ structures into a $2 \times 2 \times 2$ anti-phase modulation to further minimize the electrostatic interaction across layers[14]. This results in the overall 3D CDW order observed in neutron or X-ray scattering, for example[3,36]. Therefore, these experiments establish that the critical aspect of this problem is that *the CDW transition is driven by the action taking place within each layer*; the additional three-dimensional modulation is a somewhat minor consequence of the vertical stacking of individual $2 \times 2$ CDWs.

Consequently, a detailed study of the 2D CDW and its evolution with doping can clarify the connection between the 2D bulk order and help in provide long-sought answers related to the physics underlying the CDW instability in $TiSe_2$, bulk or monolayer. In addition, the reduced screening implies that electrons and holes in the 2D case are more strongly coupled with each other than in the 3D counterpart according to the excitonic mechanism where electron-electron interactions play a crucial role. Therefore, the 2D excitonic phase is expected to be more stable than in the 3D counterpart. This prediction (or feature) from the excitonic physics is entirely in line with the experimental observation that $T_c$ systematically increases with decreasing sample thickness[8,35].

In conclusion, since all recent experimental information concurs in that the CDW order is stabilized by the intra-layer physics, and the phase diagram is qualitatively the same as a function of doping, and quantitatively differs only in the fact that thinner samples have slightly higher $T_c$, the theoretical study of an isolated monolayer is sufficient to characterize the key microscopic details at play, even in bulk $TiSe_2$.

* Corresponding author: vpereira@nus.edu.sg

[1] H. Bruus and K. Flensberg, *Many-body quantum theory in condensed matter physics: an introduction* (Oxford University Press, 2004).

[2] L. J. Li, E. C. T. O'Farrell, K. P. Loh, G. Eda, B. Özyilmaz, and A. H. Castro Neto, Nature **529**, 185 (2015).

[3] F. J. Di Salvo, D. E. Moncton, and J. V. Waszczak, Phys. Rev. B **14**, 4321 (1976).

[4] E. Morosan, H. Zandbergen, B. Dennis, J. Bos, Y. Onose, T. Klimczuk, A. Ramirez, N. Ong, and R. Cava, Nat. Phys. **2**, 544 (2006).

[5] C. Monney, H. Cercellier, F. Clerc, C. Battaglia, E. F. Schwier, C. Didiot, M. G. Garnier, H. Beck, P. Aebi, H. Berger, L. Forró, and L. Patthey, Phys. Rev. B **79**, 045116 (2009).

[6] H. Cercellier, C. Monney, F. Clerc, C. Battaglia, L. Despont, M. G. Garnier, H. Beck, P. Aebi, L. Patthey, H. Berger, and L. Forró, Phys. Rev. Lett. **99**, 146403 (2007).

[7] C. Monney, C. Battaglia, H. Cercellier, P. Aebi, and H. Beck, Phys. Rev. Lett. **106**, 106404 (2011).

[8] P. Chen, Y. H. Chan, X. Y. Fang, Y. Zhang, M. Y. Chou, S. K. Mo, Z. Hussain, a. V. Fedorov, and T. C. Chiang, Nat. Commun. **6**, 8943 (2015).

[9] C. Monney, G. Monney, P. Aebi, and H. Beck, New Journal of Physics **14**, 075026 (2012).

[10] J. van Wezel, P. Nahai-Williamson, and S. S. Saxena, Phys. Rev. B **81**, 165109 (2010).

[11] J. van Wezel, P. Nahai-Williamson, and S. S. Saxena, EPL (Europhysics Letters) **89**, 47004 (2010).

[12] H. Frohlich, Proc. R. Soc. A Math. Phys. Eng. Sci. **215**, 291 (1952).

[13] B. Zenker, H. Fehske, H. Beck, C. Monney, and A. R. Bishop, Phys. Rev. B **88**, 075138 (2013).

[14] G. Grüner, *Density Waves in Solids* (Addison-Wesley, 1994).

[15] W. D. Wise, M. C. Boyer, K. Chatterjee, T. Kondo, T. Takeuchi, H. Ikuta, Y. Wang, and E. W. Hudson, Nat. Phys. **4**, 696 (2008).

[16] D. Mou, A. Sapkota, H.-H. Kung, V. Krapivin, Y. Wu, A. Kreyssig, X. Zhou, A. I. Goldman, G. Blumberg, R. Flint, and A. Kaminski, Phys. Rev. Lett. **116**, 196401 (2016).

[17] L. Su, C.-H. Hsu, H. Lin, and V. M. Pereira, Phys. Rev. Lett. **118**, 257601 (2017).

[18] C.-W. Chen, J. Choe, and E. Morosan, Reports Prog. Phys. **79**, 084505 (2016).

[19] A. Kogar, M. S. Rak, S. Vig, A. A. Husain, F. Flicker, Y. I. Joe, L. Venema, G. J. MacDougall, T. C. Chiang, E. Fradkin, J. van Wezel, and P. Abbamonte, Science **358**, 1314 (2017).

[20] P. Hohenberg and W. Kohn, Phys. Rev. **136**, B864 (1964).

[21] G. Kresse and D. Joubert, Phys. Rev. B **59**, 1758 (1999).

[22] G. Kresse and J. Furthmüller, Phys. Rev. B **54**, 11169 (1996).

[23] J. P. Perdew, K. Burke, and M. Ernzerhof, Phys. Rev. Lett. **77**, 3865 (1996).

[24] S. Baroni, P. Giannozzi, and A. Testa, Phys. Rev. Lett. **58**, 1861 (1987).

[25] A. Togo, F. Oba, and I. Tanaka, Phys. Rev. B **78**, 134106 (2008).

[26] N. D. Mermin, Phys. Rev. **137**, A1441 (1965).

[27] D. L. Duong, M. Burghard, and J. C. Schön, Phys. Rev. B **92**, 245131 (2015).

[28] B. Singh, C.-H. Hsu, W.-F. Tsai, V. M. Pereira, and H. Lin, Phys. Rev. B **95**, 245136 (2017).

[29] V. Popescu and A. Zunger, Phys. Rev. B **85**, 085201 (2012).

[30] W. Kohn, Phys. Rev. Lett. **19**, 439 (1967).

[31] M. Cazzaniga, H. Cercellier, M. Holzmann, C. Monney, P. Aebi, G. Onida, and V. Olevano, Phys. Rev. B **85**, 195111 (2012).

[32] A. V. Krukau, O. A. Vydrov, A. F. Izmaylov, and G. E. Scuseria, J. Chem. Phys. **125**, 224106 (2006).

[33] G. Wu, H. X. Yang, L. Zhao, X. G. Luo, T. Wu, G. Y. Wang, and X. H. Chen, Phys. Rev. B **76**, 024513 (2007).

[34] P. Chen, Y.-H. Chan, M.-H. Wong, X.-Y. Fang, M. Y. Chou, S.-K. Mo, Z. Hussain, A.-V. Fedorov, and T.-C. Chiang, Nano Lett. **16**, 6331 (2016).

[35] P. Goli, J. Khan, D. Wickramaratne, R. K. Lake, and A. A. Balandin, Nano Lett. **12**, 5941 (2012).

[36] F. Weber, S. Rosenkranz, J. P. Castellan, R. Osborn, G. Karapetrov, R. Hott, R. Heid, K. P. Bohnen, and A. Alatas, Phys. Rev. Lett. **107**, 266401 (2011).
